# Supplementary material for: Estimating Renyi Entropy of Discrete Distributions
Source: arXiv:1408.1000 source file (2016-03-10)
Supplement: Supplementary file 1 [file appendix_v4.tex]

\section*{Appendix}
\begin{replemma}{l:bound_Poisson_moments} Let $X \sim \psns \lambda$ and let $\beta$ be a positive real number. 
Then,
\[
\expectation{ X^\beta} \leq c(\beta) \max\{\lambda, \lambda^\beta\},
\]
where the constant $c(\beta)$ does not depend on $\lambda$.
\end{replemma}
\begin{proof}
For the case when $\lambda > 1$, we have
\begin{align}
\expectation{ X^\beta} &\leq  \sum_{i\leq 2\lambda} \psnlmbs i \, i^\beta + \sum_{i> 2\lambda} \psnlmbs i \, i^\beta 
\nonumber
\\
&\leq 2^\beta\lambda^\beta + \sum_{i> 2\lambda} \psnlmbs i \, i^\beta.
\nonumber
\end{align}
Using the standard tail bound for Poisson random variables, if $\lambda>1$,
for all $i > 2\lambda$
\begin{align*}
\psnlmbs i  \leq \bPr{X \geq i} \leq \exp\left(-\frac{i-\lambda}{8\lambda}\right),
\end{align*}
where the second inequality follows upon bounding the cumulant-generating function of $X$ for $i > 2\lambda$
and $\lambda>1$. Therefore, 
\begin{align}
\expectation{ X^\beta} \leq \left(2^\beta +   e^{1/8}\int e^{-x/8}x^\beta \, dx\right) \lambda^\beta,
\quad \lambda >1.
\nonumber
\end{align}
For  $\lambda \leq 1$, since $\lambda^i \leq \lambda$
for all $i \geq 1$
\begin{align}
\expectation{ X^\beta} \leq \lambda \sum_{i=1}^\infty \frac{i^\beta}{i!},
\end{align}
and the lemma follows upon choosing
\[
c(\beta) = \max\left\{ \sum_{i=1}^\infty \frac{i^\beta}{i!}, \left(2^\beta +   e^{1/8}\int e^{-x/8}x^\beta \, dx\right) \right\},
\]
which is a finite quantity.
\end{proof}
